# Supplementary material for: KV-Compress: Paged KV-Cache Compression with Variable Compression Rates per Attention Head
Source: arXiv:2410.00161 source file (2024-10-07)
Supplement: Supplementary file 1 [file appendix.tex]

\section{Llama-3.1 LongBench performance by compression rate}

% plot llama 70B code subtask performance under old prompt, with sample outputs at each compression rate.
